# Supplementary material for: Optimal Excess Risk Bounds for Empirical Risk Minimization on $p$-Norm Linear Regression
Source: arXiv:2310.12437 source file (2024-06-17)
Supplement: Supplementary file 1 [file prelims_old.tex]

In this section, we rigorously establish some basic results that we took for granted in the main paper. We start in Section \ref{subsec:apdx_degenerate} where we discuss the case where the covariates $X$ have a degenerate distribution, and show that its analysis can be directly reduced to the non-degenerate case. %In section \ref{subsec:apdx_degenerate}, we establish the differentiability properties of the risk.

\subsection{Covariates with degenerate distribution}
\label{subsec:apdx_degenerate}
Throughout the main paper, we assumed that the random vector $X$ had full support, i.e. that $\Prob\paren*{\inp{w}{X} = 0} = 1$ only if $w = 0$, and claimed that this is without loss of generality. We show why this is the case in this section. Let $X$ be an arbitrary random vector taking values in $\R^{m}$ for some $m \in \N$.

\subsection{Existence and uniqueness of minima}

\subsection{Differentiability of the risk}
In this section, we study the differentiability properties of the risk. We start by showing that under a subset of our assumptions, the risk is differentiable everywhere on $\R^{d}$.
\begin{lemma}
\label{lem:diff}
    Let $p \in (1, \infty)$ and assume that $\Exp\brack{\abs{Y}^{p}} < \infty$ and $\Exp\brack{\abs{X_j}^{p}} < \infty$ for all $j \in [d]$. Then $R_{p}$ is differentiable on all of $\R^{d}$, and
    \begin{equation*}
        \nabla R_{p}(w) = \Exp\brack{\nabla \lp(\error)}. %= \frac{1}{p-1}\Exp\brack{\sgn\paren{\error} \abs{\error}^{p-1}X}
    \end{equation*}
\end{lemma}
\begin{proof}
    We will use the dominated convergence theorem for the proof, mimicking the argument in Theorem 2.27 in \citet{follandRealAnalysisModern2013a} with a few necessary changes. Fix $w \in \R^{d}$, $j \in [d]$, let $e_j \in \R^{d}$ be the $j$-th vector of the standard basis, and define
    \begin{equation*}
        f^{j}((X, Y), t) \defeq \lp(\inp{w + te_j}{X} - Y).
    \end{equation*}
    Let $(t_n)_{n=1}^{\infty}$ be any sequence converging to zero, and define
    \begin{equation*}
        h^{j}_{n}((X, Y)) \defeq \frac{f^{j}((X, Y), t_n) - f^{j}((X, Y), 0)}{t_n}.
    \end{equation*}
    Let $t_{*} \defeq \max\brace*{\abs{t_n} \mid n \in \N}$. Note that the maximum is achieved since the sequence converges to $0$. Now $f^{j}((X, Y), t)$ is differentiable as a function of $t$, so by the mean value theorem we have
    \begin{equation*}
        \abs{h^{j}_{n}((X, Y))} \leq \sup_{t \in (-t_{*}, t_{*})} \abs*{\frac{\partial f_j}{\partial t}((X, Y), t)}
    \end{equation*}
    Furthermore, we have, for all $t \in (-t_{*}, t_{*})$
    \begin{align*}
        \abs*{\frac{\partial f^{j}}{\partial t}((X, Y), t)} &= \frac{1}{p-1} \abs*{\inp{w + te_{j}}{X}}^{p-1}\abs{X_j} \\
        &\leq \frac{\max\brace{2^{p-1}, 1}}{p-1} \brack*{\abs{\error}^{p-1}\abs{X_j} + t_{*}^{p-1} \abs{X_j}^{p}} \eqdef g(X, Y)
    \end{align*}
    where we used the inequality $\abs{a+b}^{p} \leq \max\brace{2^{p-1}, 1}(\abs{a}^{p} + \abs{b}^{p})$ in the second line valid for $p > 0$. Using Holder's inequality and our assumptions on $X$ and $Y$ we get
    \begin{equation*}
        \Exp\brack*{g(X, Y)} \leq \frac{\max\brace{2^{p-1}, 1}}{p-1} \paren*{\Exp\brack*{\abs{\error}^{p}}^{\frac{p-1}{p}} \Exp\brack*{\abs{X_j}^{p}}^{1/p} + t_{*}^{p-1} \Exp\brack*{\abs{X_j}^{p}}} < \infty
    \end{equation*}
    Applying the dominated convergence theorem on the sequence of functions $(h_{n}^{j})_{n=1}^{\infty}$ with dominating function $g$, we obtain
    \begin{align*}
        \frac{\partial R_{p}}{\partial w_j} (w) &= \lim_{n \to \infty} \frac{R_{p}(w + t_{n}e_j) - R_{p}(w)}{t_n} \\
        &= \lim_{n \to \infty} \Exp\brack*{h_{n}^{j}(X, Y)} \\
        &= \Exp\brack*{\lim_{n \to \infty} h_n^{j}(X, Y)} \\
        &= \Exp\brack*{\frac{\partial \lp}{\partial w_j}(\error)}
    \end{align*}
    where the existence of the partial derivative of $R_{p}$ is justified by the above computation. A similar argument may be used to show that the partial derivative function $\brace*{\partial R_{p} / \partial w_j}(w)$ is continuous, proving that $R_{p}$ is differentiable with the stated formula for its gradient.
\end{proof}

We now turn to the twice differentiability of the risk. We start with the easy case $p \in [2, \infty)$.
\begin{lemma}
\label{lem:twice_diff_pgeq2}
    Let $p \in [2, \infty)$ and assume that $\Exp\brack{\abs{Y}^{p}} < \infty$ and $\Exp\brack{\abs{X_j}^{p}} < \infty$ for all $j \in [d]$. Then $R_{p}$ is twice differentiable on all of $\R^{d}$, and
    \begin{equation*}
        \nabla^{2} R_{p}(w) = \Exp\brack{\nabla^{2} \lp(\error)}
    \end{equation*}
\end{lemma}
\begin{proof}
    The proof follows from a very similar argument to the one used for Lemma \ref{lem:diff}.
\end{proof}

The case $p \in (1, 2)$ is more complicated. The following lemma establishes the twice differentiability of the risk at its minimizer under a subset of the assumptions of Theorem \ref{thm:pleq2}.
\begin{lemma}
    Let $p \in (1, 2)$. Assume that $\Prob\paren*{\abs{\opterror} = 0} = 0$ and $\Exp\brack{\abs{\opterror}^{p-2}X_j^{2}} < \infty$ for all $j \in [d]$. Then $R_{p}$ is twice differentiable at $\opt$ and
    \begin{equation*}
        \nabla^{2} R_{p}(\opt) = \Exp\brack{\nabla^{2} \lp(\opterror)}
    \end{equation*}
\end{lemma}
\begin{proof}
    The difficulty in the proof compared to Lemma \ref{lem:diff} and Lemma \ref{lem:twice_diff_pgeq2} stems from the fact that the loss is not twice differentiable at zero. We still rely on the dominated convergence theorem, but the construction of the dominating function is slightly more intricate.

    We start as in the proof of Lemma \ref{lem:diff}. Let $i, j \in [d]$, and let $e_i$ be the $i$-th vector of the standard basis. Define
    \begin{equation*}
        f^{ji}((X, Y), t) \defeq \frac{1}{p-1} \sgn\paren*{\inp{\opt + t e_{i}}{X} - Y} \abs{\opterror}^{p-1} X_j
    \end{equation*}
    Let $(t_n)_{n=1}^{\infty}$ be any sequence that converges to zero, and define
    \begin{equation*}
        h^{ji}_{n}((X, Y)) \defeq \frac{f^{ji}((X, Y), t_n) - f^{ji}((X, Y), 0)}{t_{n}}
    \end{equation*}
    Our goal is to construct a dominating integrable function for the sequence $(h^{ji}_{n})_{n=1}^{\infty}$. We split this problem into two cases. First, assume that $\abs{t_{n}} > \abs{\opterror}/\paren*{2 \abs{X_i}}$. Then
    \begin{align}
        \abs{h_{n}^{ji}((X, Y))} &\leq \frac{\abs{f^{ji}((X, Y), t_{n})} + \abs{f^{ji}((X,Y), 0)}}{\abs{t_n}} \nonumber \\
        &= \frac{1}{p-1} \frac{\paren*{\abs{\inp{\opt + te_i}{X} - Y}^{p-1} + \abs{\inp{\opt}{X} - Y}^{p-1}}\abs{X_j}}{\abs{t_n}} \nonumber \\
        &\leq \frac{1}{p-1} \paren*{\frac{2 \abs{\opterror}^{p-1}\abs{X_j}}{\abs{t_n}} + \abs{t_{n}}^{p-2} \abs{X_i}^{p-1}\abs{X_{j}}} \nonumber \\
        &\leq \frac{8}{p-1} \abs*{\opterror}^{p-2} \abs{X_i}\abs{X_j} \label{eq:ineq71}
    \end{align}
    where the second inequality follows from $\abs{a+b}^{p} \leq \abs{a}^{p} + \abs{b}^{p}$ valid for $p \in (0, 1)$, and the last by using the lower bound assumed on $t_{n}$. In the second case, we have $\abs{t_{n}} \leq \abs{\opterror}/\paren*{2 \abs{X_i}} \eqdef t^{*}(X, Y)$, from which we deduce that
    \begin{equation*}
        \abs{\inp{\opt + t_{n} e_i}{X} - Y} \geq \abs{\opterror} - t_{n}\abs{X_i} \geq \frac{\abs{\opterror}}{2} > 0,
    \end{equation*}
    so that $f^{ij}((X, Y), t)$ is differentiable as a function of $t$ on $(-t^{*}(X, Y), t^{*}(X, Y))$. By the mean value theorem, we obtain
    \begin{equation}
    \label{eq:ineq72}
        \abs{h_n^{ij}((X, Y))} \leq \sup_{t \in (-t^{*}(X, Y), t^{*}(X, Y))} \abs*{\frac{\partial f^{ji}}{\partial t}((X, Y), t)} \leq 2 \abs{\opterror}^{p-2} \abs{X_j}\abs{X_i}
    \end{equation}
    Combining inequalities (\ref{eq:ineq71}) and (\ref{eq:ineq72}), we define our dominating function
    \begin{equation*}
        g(X, Y) \defeq \frac{16}{p-1} \abs{\opterror}^{p-2} \abs{X_{i}}\abs{X_{j}} \leq \frac{8}{p-1} \abs{\opterror}^{p-2} (X_{i}^{2} + X_{j}^{2})
    \end{equation*}
    where we used $2ab \leq a^{2} + b^{2}$. Using our assumptions, it is clear that $g(X, Y)$ is integrable. Applying the dominated convergence theorem as in Lemma \ref{lem:diff} yields the result.
\end{proof}

\iffalse
\begin{proof}
    Note that for any $w \in \R^{d}$, $\lp(\error)$ is twice differentiable at $w$ if and only if $\error \neq 0$. Therefore, by assumption, we have that $\lp(\error)$ is almost surely twice differentiable at $\opt$ with partial derivatives
    \begin{equation*}
        \frac{\partial^{2} \lp(\error)}{\partial w_j\partial w_i} = \abs{\error}^{p-2}X_jX_i
    \end{equation*}
    for all $i, j \in [d]$. For $j \in [d]$, we have, by assumption
    \begin{equation*}
        \Exp\brack*{\abs*{\frac{\partial^{2} \lp(\error)}{\partial w_j^{2}}}} = \Exp\brack*{\abs{\error}^{p-2} X_{j}^{2}} < \infty
    \end{equation*}
    and for $i,j \in [d]$ with $i \neq j$ we have:
    \begin{equation*}
        \Exp\brack*{\abs*{\frac{\partial^{2} \lp(\error)}{\partial w_j\partial w_i}}} = \Exp\brack*{\abs{\error}^{p-2} \abs{X_{i} X_{j}}} \leq \frac{1}{2} \Exp\brack*{\abs{\error}^{p-2} (X_{i}^2 + X_{j}^{2})} < \infty
    \end{equation*}
    where we used the inequality $2ab \leq a^{2} + b^{2}$ for the first inequality, and our assumption for the second. Applying Theorem 2.27 in \citet{follandRealAnalysisModern2013a} as in the proof of Lemma \ref{lem:diff} completes the proof.
\end{proof}
\fi
